# Supplementary material for: Estimating the Longest Increasing Subsequence in Nearly Optimal Time
Source: arXiv:2112.05106 source file (2022-11-01)
Supplement: Supplementary file 1 [file appendix.tex]

\section{Algorithm for finding multiple $\LIS$}

\begin{theorem}
Consider an instance $\cE$
\end{theorem}

\subsection{Old}

\aanote{TO REMOVE?}

We note that a brute force search for $\LIS$ will take $O(n\cdot k^2 / \lambda)$ time, which is prohibitive for our fine-grained application. We hence devise the following parallel $\LIS$ approximation algorithm.

We call the below initially with $U = [n] \times [k]$ and iterate it with all $\lambda' \in 1/E_2(1/\lambda)$.

\blue{Intuition: The idea is that if there are many disjoint (non-overlapping) pseudo solutions of a certain range, there are many combinations as well, then splitting them into buckets we can still find pseudo solutions with almost same length, hence we never have to brute force too many (i think $\log(nk)$ overhead only)}
\newcommand{\fs}{\textsc{Finding-Solutions}}
\subsection{Algorithm Description}
\paragraph{\fs($g,U,\lambda$)}
\begin{enumerate}
    \item If $|U| \leq O(n \log^{O(1)}(nk))$, compute and return all solutions of length at least $\lambda n$ in $U'$ using the algorithm in \cite{rubinstein2019approximation}.
    \item Let $U_1, U_2$ be an iid coin-flip partition of $U$.
    \item $\cS_1 \gets \textsc{Finding-Solutions}(g,U_1,\lambda(1-\delta))$.
    \item $\cS_2 \gets \textsc{Finding-Solutions}(g,U_2,\lambda(1-\delta))$.
    \item $U' \gets U \setminus (\cS_1 \cup \cS_2$).
   % \begin{enumerate}
        \item Compute $\polylog(nk)$ solutions of length at least $\lambda n$ in $U'$ using the algorithm in \cite{rubinstein2019approximation}; let $\cS'$ be this set of such solutions.
        \item If there are no more solutions left, return $\cS' \cup \cS_1 \cup \cS_2$.
        
%        \item If $|\cS_1 \cup \cS_2| > |U|/\Theta(\polylog nk)$, return $\cS_1 \cup \cS_2 \cup \textsc{Finding-Solutions}(g,U',\lambda)$.    
\item Otherwise, return $\cS_1 \cup \cS_2 \cup \cS' \cup \textsc{Finding-Solutions}(g,U' \setminus \cS',\lambda)$.
        %If there are any 
        %\nnote{we may need to stop after $\log (nk)$ solutio%ns are found, then find the rest at the next $\lambda$ for some extremal cases...}.
  %      \item return $\cS' \cup \cS_1 \cup \cS_2$.
  %  \end{enumerate}
    
\end{enumerate}

\subsection{Correctness}

\begin{claim}
    Let $p \subset U$ be a solution. Then at least one of $U_1$ and $U_2$ contains an increasing subsequence of $p$ of length at least at least $|p|/2$.
\end{claim}

\begin{proof}
    This is immediate from the fact that $\{U_1,U_2\}$ is a partition of $U$.
\end{proof}

\begin{corollary}
    The recursion depth of $\fs$ is at most $O(\polylog (nk))$
\end{corollary}

\begin{claim}
    Suppose any (balanced?) set of coordinates $U$ has at least $s$ disjoint solutions of length $\geq|p|$. Then if we subsample $\tilde{U}$ with probability $q > 1/3$, we find w.h.p  $q(1-\delta)s$ disjoint solutions of length at least $\alpha|p|$, where $\alpha > 1-\tfrac{1}{\log nk}$.
\end{claim}

\subsection{Time complexity}
%\ns{Formally define the inputs to the $\genlis$ and $\reslis$ problems...}

%\ns{Amend $\reslis$ algorithm to discretize over $Y$ and fix $|X_i|
%$}

%\ns{prove main theorem in section 5 - Alex is this done??}

% add the fast decay over reslis recursive steps...}

%\ns{Formalize better parameter $k$}

%\ns{Prove 4.3! [Sandip] 4.1 as well?}

%\ns{state and analyze run-time for all algorithms!}

%\ns{finish the proof of Section 7 - $r^*$ vs $\rho^*$}

%\ns{border issues...}

%\ns{unify notations. for example OPT vs $X^*$, etc... - mostly done, rest is of low priority}
